# Supplementary material for: Calculating the Magnetic Anisotropy of Rare-Earth-Transition-Metal Ferrimagnets
Source: arXiv:1803.00235 source file (2018-03-01)
Supplement: Supplementary file 1 [file supplemental.pdf]

# Calculating the magnetic anisotropy of rare-earth/transition-metal ferrimagnets: Supplemental Material

Christopher E. Patrick,[1,*] Santosh Kumar,[1] Geetha Balakrishnan,[1] Rachel S. Edwards,[1] Martin R. Lees,[1] Leon Petit,[2] and Julie B. Staunton[1]

[1]*Department of Physics, University of Warwick, Coventry CV4 7AL, United Kingdom*

[2]*Daresbury Laboratory, Daresbury, Warrington WA4 4AD, United Kingdom*

(Dated: January 30, 2018)

## COMPUTATIONAL DETAILS

Electronic structure calculations were carried out using the Korringa-Kohn-Rostoker (KKR) formulation of DFT, using an adaptive reciprocal space sampling for high numerical precision [1] and performing the finite temperature statistical averaging within the coherent potential approximation [2]. The single-site problem was solved fully-relativistically via the Dirac-Kohn-Sham equation [3] using the atomic-sphere approximation and frozen potentials determined in scalar-relativistic calculations (using the `Hutsepot` code [4]) on the fully ordered magnetic system. We used the local-spin-density approximation for the exchange-correlation energy [5] and further treated the Gd-4$f$ electrons with the local self-interaction correction [6]. We used the same lattice parameters, atomic sphere radii, core-valence partitioning and energy integration contours as in Ref. [7], and refer the reader to that work for a more in-depth discussion of the disordered local moment picture.

## IMPLEMENTATION OF THE ORBITAL POLARIZATION CORRECTION

The orbital polarization correction (OPC) was introduced as a means of accounting for Hund's second rule in DFT [8]. In general, approximate exchange correlation functionals which only depend on the electron spin-density do not enforce this rule, requiring a current-density formulation [9]. Practically the OPC is an orbital-dependent potential which enters the single-particle Hamiltonian [10]:

$$\hat{H}_{\mathrm{OPC}} = \sum_i \sum_{lm\sigma} -B_{l\sigma} \langle \hat{l}_z \rangle_\sigma m \hat{P}^i_{lm\sigma} \tag{1}$$

Here, $\hat{P}^i_{lm\sigma}$ is a projector onto the atom labelled $i$, the angular momentum channel $lm$ and the spin channel $\sigma$, and $\hat{l}_z$ is the operator for the third component of the orbital momentum. The expectation value $\langle \hat{l}_z \rangle_\sigma$ is calculated projecting onto a spin channel $\sigma$. $B_{l\sigma}$ is the Racah parameter built from the spherically-symmetric charge density with angular momentum and spin character $l, \sigma$.

The fact that the expectation value appears in the potential means that the correction must be determined self-consistently. Our strategy to incorporate the OPC into our disordered-local moment calculations is to calculate self-consistently the OPC potential once for the ordered magnetic state aligned along the $c$-axis (for $GdCo_5$, the Gd moments are antialigned to Co). This same OPC potential is then used for the disordered calculations. This approach is consistent with our "frozen potential" approach.

We apply the OPC to the $d$ channel, and for simplicity use two distinct Racah parameters only; 77 meV for R and 150 meV for Co (the same for both spin channels). These values were chosen based on those reported in Ref. [10]. The corresponding self-consistent values of $\langle \hat{l}_z \rangle_\sigma$ are $(\langle \hat{l}_z \rangle_{\sigma_\uparrow}, \langle \hat{l}_z \rangle_{\sigma_\downarrow})$ = (-0.03,0.32) and (-0.04,0.22) for the two inequivalent Co sites in $YCo_5$, and (-0.04,0.35) and (-0.05,0.23) for Co in $GdCo_5$ (here, $\uparrow$ denotes the majority spin direction of the Co atoms). $\langle \hat{l}_z \rangle_\sigma$ was found to be very small for R, e.g. (0.07,-0.08) for Gd.

Equation 1 is written in terms of the $(l, m, \sigma)$ quantum numbers, which are a natural basis for scalar-relativistic calculations. To incorporate this correction into the relativistic Kohn-Sham-Dirac equation we broadly follow Refs. [11] and [12]. It is convenient to introduce the matrix

$$\tilde{V}_{\mathrm{OPC}} = \begin{pmatrix} \hat{H}_{\mathrm{OPC}} & 0 \\ 0 & \hat{H}_{\mathrm{OPC}} \end{pmatrix}. \tag{2}$$

Due to the spin-projector in $\hat{H}_{\text{OPC}}$, $\tilde{V}_{\text{OPC}}$ acts on bispinors and can therefore be inserted directly into the Kohn-Sham-Dirac equation. The equation can then be solved using the standard procedure using a basis of spin-angular functions $|\kappa, m_j\rangle$ [13], which requires matrix elements of the form

$$\mathcal{G}^{m_j}(\kappa_1, \kappa_2) = \langle \kappa_1, m_j | \hat{H}_{\text{OPC}} | \kappa_2, m_j \rangle. \tag{3}$$

Evaluating the projector term $\langle \kappa_1, m_j | \hat{P}^i_{lm\sigma} | \kappa_2, m_j \rangle$ finds most $\kappa_1, \kappa_2$ combinations are zero, except for those belonging to the same $l$ ($\kappa_1 = \kappa, \kappa'; \kappa_2 = \kappa, \kappa'; \kappa = -l-1, \kappa' = l$). This situation is the same as for the spin-coupling to the effective exchange-correlation magnetic field, so introducing the OPC does not lead to new couplings [12]. Rather the existing coupled equations gain an extra term involving $B_{l\sigma} m \langle \hat{l}_z \rangle_\sigma$ and products of Clebsch-Gordan coefficients. Incorporating this extra term requires some careful bookkeeping but constitutes only a small modification to our existing relativistic single-site solver.

## DERIVATION OF THE SUCKSMITH-THOMPSON EQUATION

Equation 1 of the main text was derived in Ref. [14] starting from the following model free energy:

$$\begin{aligned} F_{\mathrm{ST}}(\theta) &= \kappa_1 \sin^2\theta + \kappa_2 \sin^4\theta - \boldsymbol{B}\cdot\boldsymbol{M} \\ &= \kappa_1 \sin^2\theta + \kappa_2 \sin^4\theta - M_0 B\cos(\theta-\gamma) \end{aligned} \tag{4}$$

where $\theta$ and $\gamma$ are the angles with respect to the easy axis of the magnetization $\boldsymbol{M}$ and field $\boldsymbol{B}$ respectively, and $\kappa_1$, $\kappa_2$ are the anisotropy constants. Applying the field in the hard plane ($\gamma = \pi/2$) and differentiating with respect to $\theta$ gives

$$\begin{aligned} \frac{dF_{\mathrm{ST}}}{d\theta} &= 2\kappa_1 \sin\theta\cos\theta + 4\kappa_2 \sin^3\theta\cos\theta - M_0 B\cos\theta \\ &= \cos\theta(2\kappa_1\sin\theta + 4\kappa_2\sin^3\theta - M_0 B). \end{aligned} \tag{5}$$

Using that the magnetization measured in the $ab$ plane $M_{\mathrm{ab}} = M_0 \sin\theta$ shows that there is a stationary point, which corresponds to a minimum of $F_{\mathrm{ST}}$ at low fields, at which

$$2\kappa_1(M_{\mathrm{ab}}/M_0) + 4\kappa_2(M_{\mathrm{ab}}/M_0)^3 - M_0 B = 0 \tag{6}$$

which after rearrangement gives

$$(BM_0/2)/\left(M_{\mathrm{ab}}/M_0\right) \equiv \eta = \kappa_1 + 2\kappa_2\left(M_{\mathrm{ab}}/M_0\right)^2. \tag{7}$$

as found in the main text.

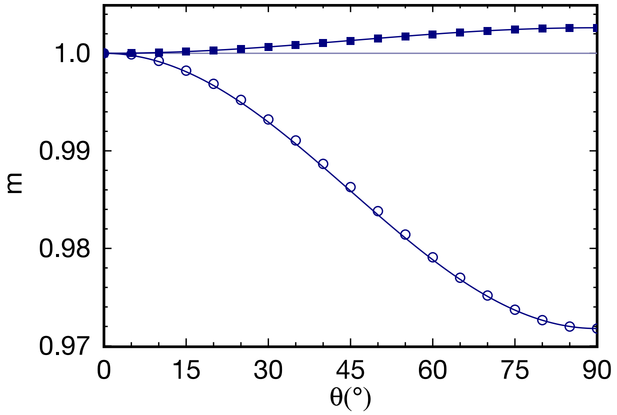


FIG. 1. Reduced magnetization $M(\theta)/M_0$ for the Gd (squares) and Co (circles) sublattices of $GdCo_5$ at 0 K. The lines are fits with the expression $1-p\sin^2\theta$ with $p_{\mathrm{Co}} = 0.028$ and $p_{\mathrm{Gd}} = -0.003$.

## MAGNETIZATION ANISOTROPY

As stated in the main text we simulate $M\mathrm{v}B$ curves from model free energy expressions by minimizing $F_{1(2)} - \sum_i \boldsymbol{M_i} \cdot \boldsymbol{B}$ with respect to the angles $\theta_{\mathrm{Gd}}$ and $\theta_{\mathrm{Co}}$. Our calculations with the Co and Gd moments held rigidly antiparallel reveal a pronounced anisotropy on the Co moments, which is well-described by $M_{\mathrm{Co}}(\theta_{\mathrm{Co}}) = M^0_{\mathrm{Co}}[1 - p\sin^2\theta_{\mathrm{Co}}]$ (Fig. 1). The anisotropy on the Gd moments is found to be an order of magnitude smaller.. Therefore the full expression that we minimize is

$$F^{\mathrm{Tot}}_{1(2)}(\theta_{\mathrm{Gd}}, \theta_{\mathrm{Co}}, B, \gamma) = F_{1(2)}(\theta_{\mathrm{Gd}}, \theta_{\mathrm{Co}}) + BM_{\mathrm{Gd}}\cos(\theta_{\mathrm{Gd}} - \gamma) - BM^0_{\mathrm{Co}}\cos(\theta_{\mathrm{Co}} - \gamma)[1 - p\sin^2\theta_{\mathrm{Co}}] \tag{8}$$

with the geometry defined in Fig. 2 of the main text.

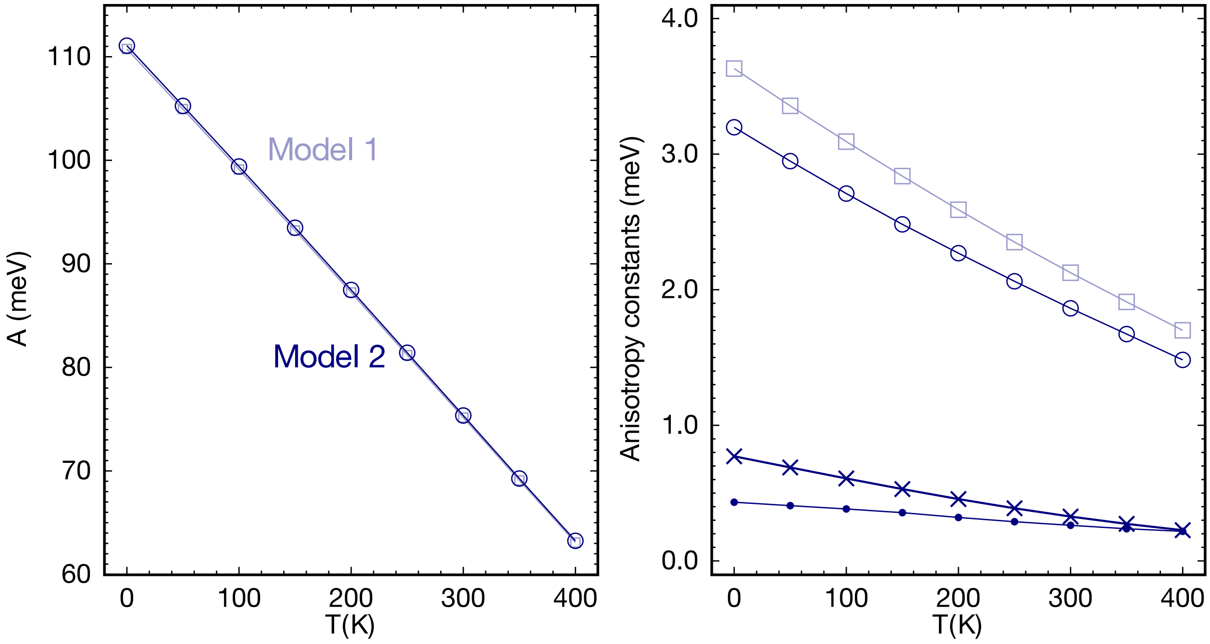


FIG. 2. Inter-sublattice exchange constants $A$ and anisotropy constants $K_{1,\mathrm{Co}}$ for the model free energies $F_1$ (equation 9, faint blue squares) and $F_2$ (equation 14, dark blue circles). For $F_2$, $K_{2,\mathrm{Co}}$ (small filled circles) and $K_{1,\mathrm{Gd}}$ (crosses) are also shown. The lines joining the points are guides to the eye. Clearly the values of $A$ calculated for $F_1$ and $F_2$ are very similar.

## CALCULATED PARAMETERS USED TO SIMULATE $M$ v $B$ CURVES

### $GdCo_5$, first model

For our first model of the free energy of $GdCo_5$, we use a slightly-modified two-sublattice expression [15]:

$$F_1(\theta_{\mathrm{Gd}}, \theta_{\mathrm{Co}}) = -A\cos(\theta_{\mathrm{Gd}} - \theta_{\mathrm{Co}}) + K_{1,\mathrm{Co}}\sin^2\theta_{\mathrm{Co}} + S(\theta_{\mathrm{Gd}}, \theta_{\mathrm{Co}}). \tag{9}$$

Here $A$ accounts for inter-sublattice exchange and $K_{1,\mathrm{Co}}$ the MCA of the cobalt sublattice. $S$ is the contribution to the anisotropy from the dipole-dipole interaction [16]:

$$S(\theta_{\mathrm{Gd}}, \theta_{\mathrm{Co}}) = S_1\sin^2\theta_{\mathrm{Gd}} + S_2\sin^2\theta_{\mathrm{Co}} + S_3\left(\sin\theta_{\mathrm{Gd}}\sin\theta_{\mathrm{Co}} - \frac{2}{3}\cos(\theta_{\mathrm{Gd}} - \theta_{\mathrm{Co}})\right). \tag{10}$$

We have isolated $S(\theta_{\mathrm{Gd}}, \theta_{\mathrm{Co}})$ because it is not included in our DFT formalism [13]. Therefore according to the model the torques on the two sublattices that we obtain from our DFT-DLM calculations are functions of $A$ and $K_{1,\mathrm{Co}}$ only:

$$\frac{\partial F}{\partial \theta_{\mathrm{Gd}}} = A\sin(\theta_{\mathrm{Gd}} - \theta_{\mathrm{Co}}) \tag{11}$$

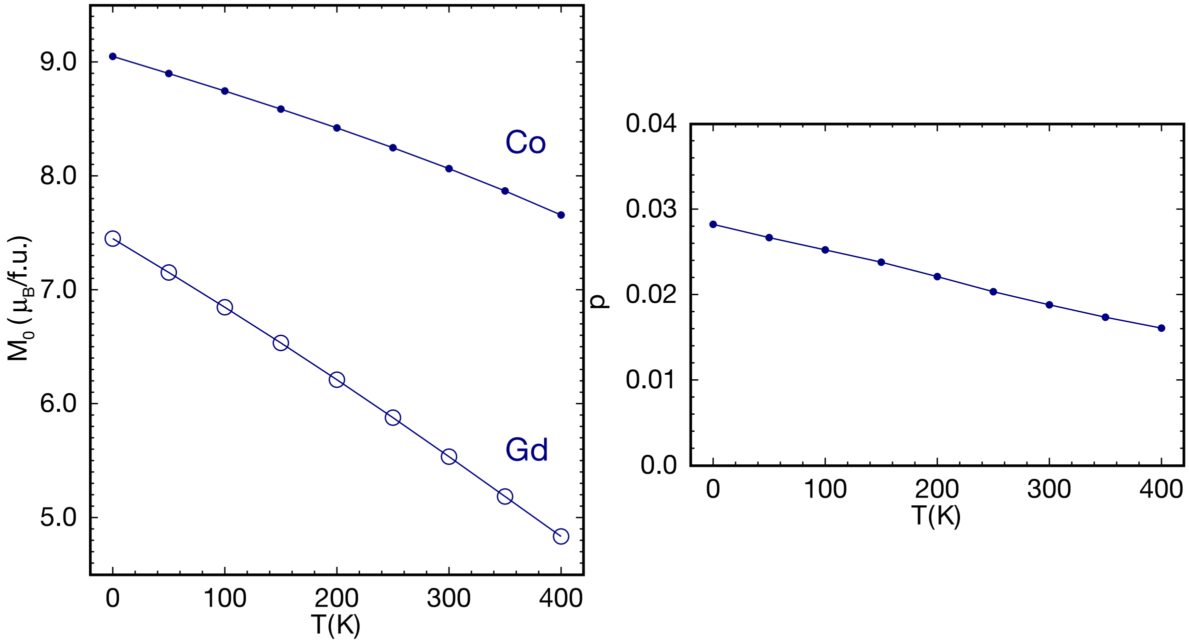


FIG. 3. Magnetizations $M_{\rm Gd}$ and $M^0_{\rm Co}$ (left panel, empty and filled circles respectively) and cobalt magnetization anisotropy (right panel) obtained for $GdCo_5$. The lines joining the points are guides to the eye.

$$\frac{\partial F}{\partial \theta_{\rm Co}} = -A \sin(\theta_{\rm Gd} - \theta_{\rm Co}) + K_{1,\rm Co} \sin(2\theta_{\rm Co}). \tag{12}$$

We constructed a training set of 28 calculations:

$$\theta_{\rm Gd} = 10°; \theta_{\rm Co} = -5°, -4°, ..., 5°$$

$$\theta_{\rm Gd} = 80°; \theta_{\rm Co} = 75°, 76°, ..., 85°$$

$$\theta_{\rm Gd} = \theta_{\rm Co} = 10°, 20°, ..., 80°$$

and obtained $A$ and $K_{1,\rm Co}$ from a least-squares fit of the torques. We show these values as the faint data points in Fig. 2.

To calculate $M_{\rm Gd}$, $M^0_{\rm Co}$ and $p$ (equation 8) we used the set of calculations with

$$\theta_{\rm Gd} = \theta_{\rm Co} = 0°, 10°, 20°, ..., 90°.$$

The extracted values are given in Fig. 3.

Finally to calculate the dipole-dipole interaction energy we use the expression

$$E_{\rm dip}(\{\theta_i\}) = -\frac{1}{2}\frac{\mu_0}{4\pi} \sum_{j\neq i} \sum_i \frac{3(\boldsymbol{M_i} \cdot \boldsymbol{R_{ij}})(\boldsymbol{M_j} \cdot \boldsymbol{R_{ij}}) - R^2_{ij} \boldsymbol{M_i} \cdot \boldsymbol{M_j}}{R^5_{ij}} \tag{13}$$

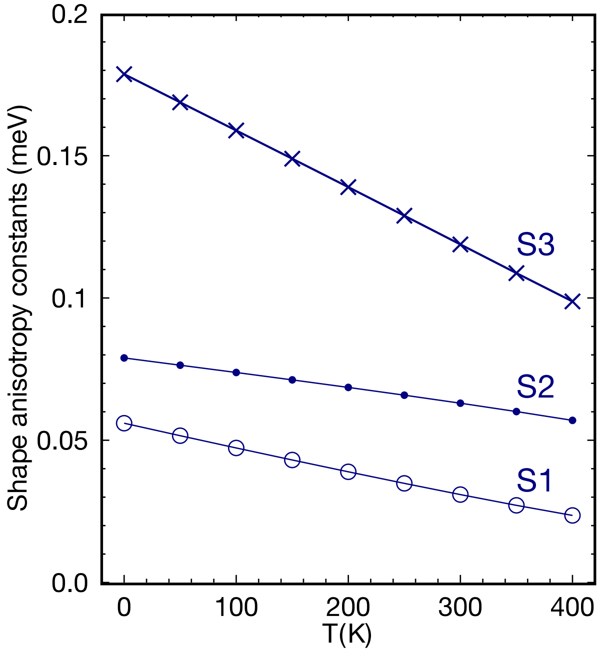


FIG. 4. Constants describing the dipole-dipole interaction energy (equation 10) calculated from equation 13.

where the atoms $i$ lie in the unit cell and $j$ includes all moments within a sphere of radius of 20 nm. We calculated $E_{\mathrm{dip}}(\{\theta_i\})$ for angle pairs ranging from 0–10° to fit $S_1, S_2, S_3$, using the temperature-dependent magnetizations $M_{\mathrm{Gd}}, M_{\mathrm{Co}}$ (note that we account for the different size of the magnetization on the two Co sublattices). Fig. 4 shows the parameters calculated over the temperature range 0–400 K.

**$GdCo_5$, second model**

As discussed in the main text we extended the free energy expression in equation 9 to account for additional angular dependences:

$$F_2(\theta_{\mathrm{Gd}}, \theta_{\mathrm{Co}}) = F_1(\theta_{\mathrm{Gd}}, \theta_{\mathrm{Co}}) + K_{2,\mathrm{Co}} \sin^4 \theta_{\mathrm{Co}} + K_{1,\mathrm{Gd}} \sin^2 \theta_{\mathrm{Gd}}. \tag{14}$$

Accordingly the torque expressions that we fit the DFT-DLM calculations to are modified:

$$\frac{\partial F}{\partial \theta_{\mathrm{Gd}}} = A \sin(\theta_{\mathrm{Gd}} - \theta_{\mathrm{Co}}) + K_{1,\mathrm{Gd}} \sin(2\theta_{\mathrm{Gd}}) \tag{15}$$

$$\frac{\partial F}{\partial \theta_{\mathrm{Co}}} = -A \sin(\theta_{\mathrm{Gd}} - \theta_{\mathrm{Co}}) + K_{1,\mathrm{Co}} \sin(2\theta_{\mathrm{Co}}) + 4K_{2,\mathrm{Co}} \sin^3 \theta_{\mathrm{Co}} \cos \theta_{\mathrm{Co}}. \tag{16}$$

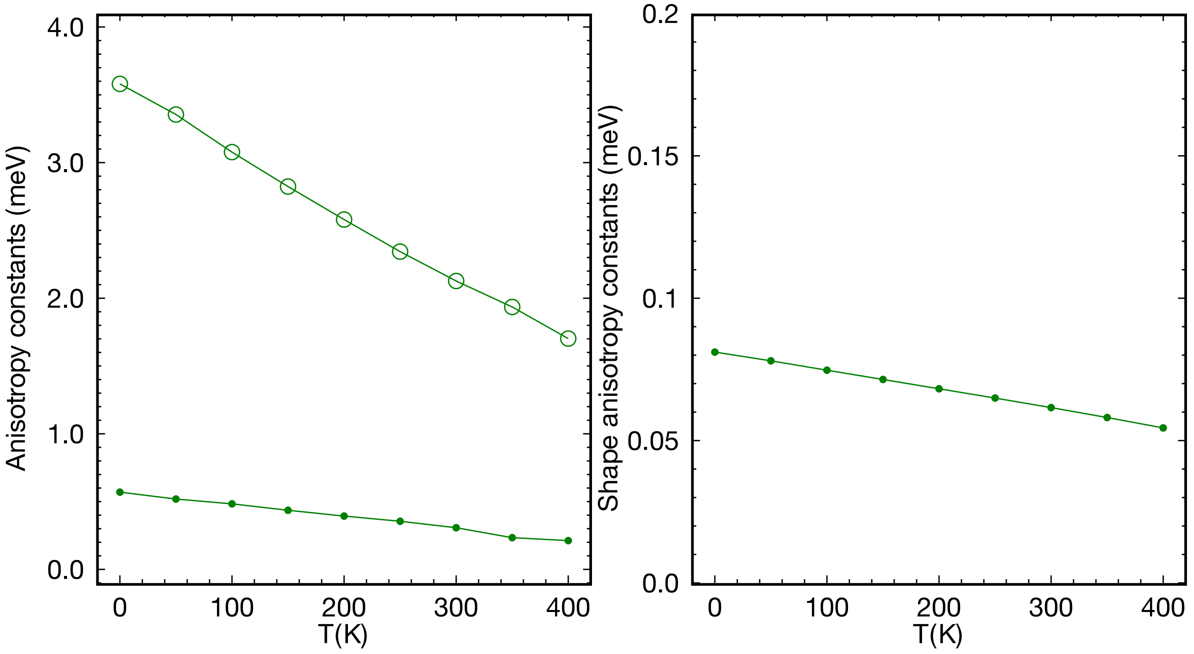


FIG. 5. Constants parametrizing the free energy of $YCo_5$ (equation 17) with the left panel showing $K_{1,\mathrm{Co}}$ and $K_{2,\mathrm{Co}}$ (empty and filled circles, respectively) and the right panel showing the dipolar contribution $S$.

However the determination of $M_{\mathrm{Gd}}$, $M^0_{\mathrm{Co}}$, $p$ and $S_1, S_2, S_3$ is unchanged. The same training set of 28 calculations are used to obtain these parameters, which are shown in Fig. 2.

### $\mathbf{YCo_5}$

We model the free energy of $YCo_5$ using the expression of Ref. [17], again separating out the dipolar term:

$$F_{\mathrm{YCo_5}}(\theta_{\mathrm{Co}}) = K_{1,\mathrm{Co}} \sin^2 \theta_{\mathrm{Co}} + K_{2,\mathrm{Co}} \sin^4 \theta_{\mathrm{Co}} + S \sin^2 \theta_{\mathrm{Co}}. \tag{17}$$

Including the magnetization anisotropy of the Co moments, the total free energy that we minimize is

$$F^{\mathrm{Tot}}_{\mathrm{YCo_5}}(\theta_{\mathrm{Co}}, B, \gamma) = F_{\mathrm{YCo_5}}(\theta_{\mathrm{Co}}) - BM^0_{\mathrm{Co}} \cos(\theta_{\mathrm{Co}} - \gamma)[1 - p \sin^2 \theta_{\mathrm{Co}}]. \tag{18}$$

We parametrize all the constants using the set of calculations $\theta_{\mathrm{Co}} = 0°, 10°, 20°, ..., 90°$ (using equation 13 for $S$). The calculated parameters are shown in Figs. 5 and 6.

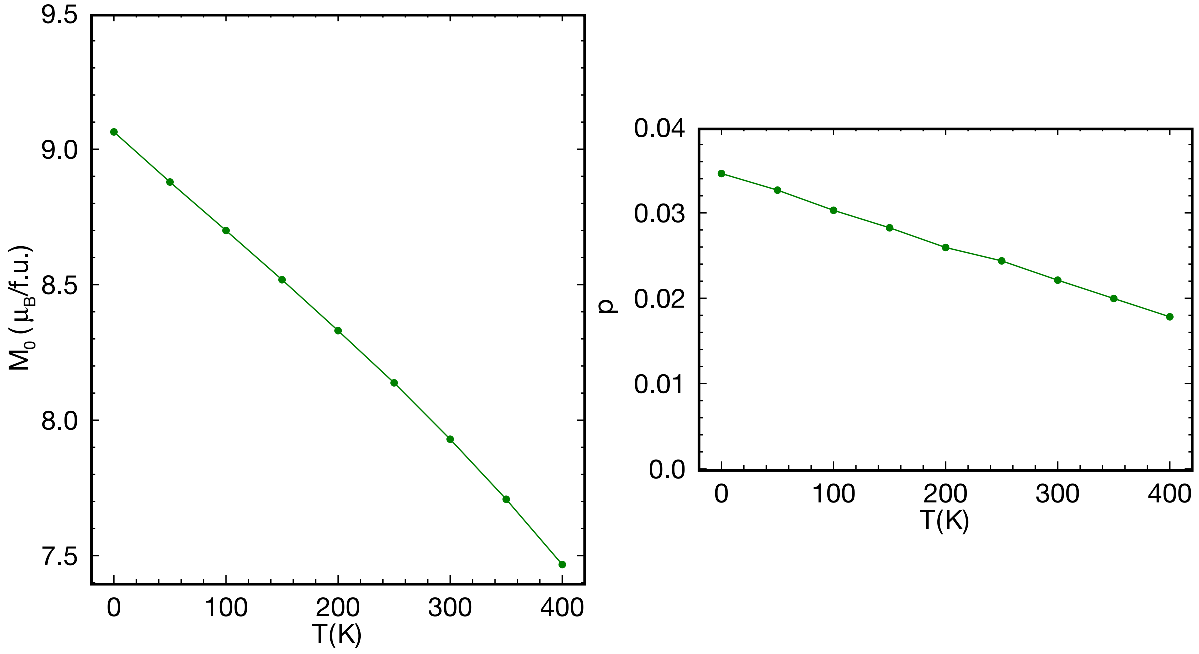


FIG. 6. Cobalt magnetization $M_{\mathrm{Co}}$ (left panel) and magnetization anisotropy $p$ (right panel) of $YCo_5$. Note the scale of the magnetization plot is different to Fig. 3.

## CALCULATION OF $M$ v $B$ CURVES BY MATCHING TORQUES

In the main text, two methods of calculating $M$v$B$ curves are introduced based on balancing the torques arising from the external field with the "internal" torques, i.e from exchange and anisotropy. Then,

$$\frac{\partial}{\partial \theta_i}\left(F(T) - \sum_j \boldsymbol{M_j} \cdot \boldsymbol{B}\right) = \frac{\partial}{\partial \theta_i}\left(F(T) - \sum_j M_j B \cos(\theta_j - \gamma)\right)$$
$$= \frac{\partial}{\partial \theta_i}\left(F(T) - \sum_j M_j B \sin\theta_j\right) = 0 \qquad (19)$$

where the second line is appropriate for the magnetic field applied in the hard plane ($\gamma = 90°$; see Fig. 2 of the text). Method (i) neglects any contribution to the torque from magnetization anisotropy, giving the condition for balancing the torque as:

$$B = \frac{\partial F(T)}{\partial \theta_i} \frac{1}{M_i \cos\theta_i}. \qquad (20)$$

Method (ii) instead treats this contribution approximately, giving the condition for balancing the torque as:

$$B = \frac{\partial F(T)}{\partial \theta_i} \frac{1}{M_i \cos\theta_i + \sin\theta_i \frac{\partial M_i}{\partial \theta_i}}, \qquad (21)$$

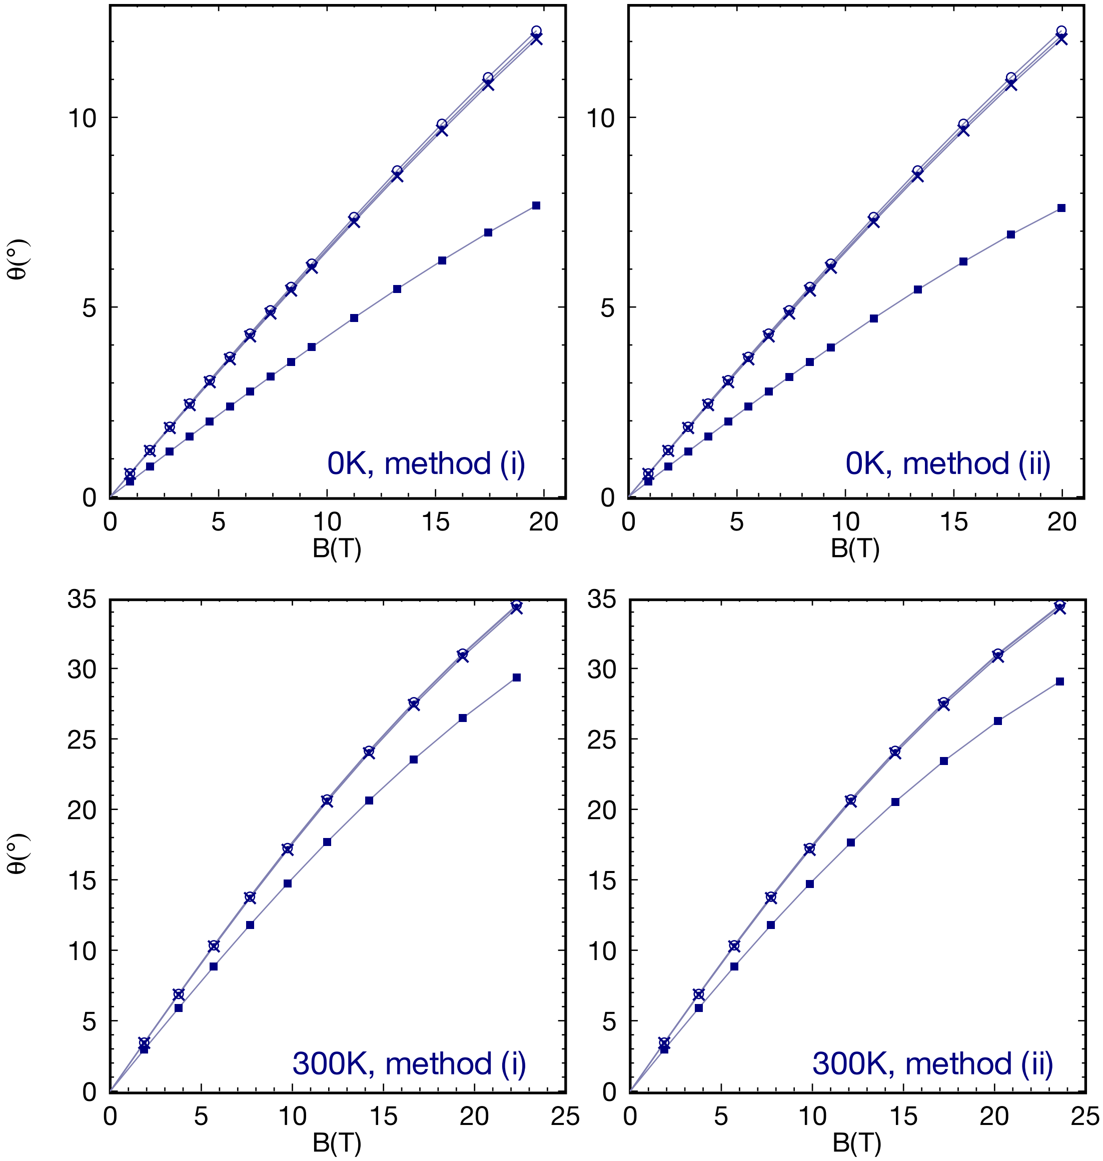


FIG. 7. Angles of Gd and Co sublattices which satisfy equation 20 [for method (i)] or equation 21 [for method (ii)] at 0 and 300 K; see Fig. 2 of main text for geometry. The filled squares represent $\theta_{\mathrm{Gd}}$, the circles the angles of the Co moments at the $2c$ sites, and the crosses and filled circles the angles of the two inequivalent moments at the $3g$ sites.

with $M_i(\theta_i) = M_{0i}(1 - p_i \sin^2\theta_i)$. $\frac{\partial F(T)}{\partial \theta_i}$ is calculated as the sum of the torque obtained from the DFT-DLM calculations with the dipole contribution, obtained numerically from equation 13. The individual magnetization anisotropies $p_i$ were obtained from the same calculations used to determine $p$.

As stated in the main text there are four distinct angles in $GdCo_5$, corresponding to

Gd, the two Co atoms occupying the $2c$ positions, two of the Co atoms occupying the $3g$ positions, and the remaining Co atom at the other $3g$ position (the symmetry of the $3g$ sites is broken when the magnetization is directed away from the $c$ axis). The angles sets which satisfy equations 20 and 21 for different fields at 0 and 300 K are shown in Fig. 7. The canting between the Gd sublattice (filled squares) and Co sublattices (other symbols) is apparent; the canting within the Co sublattices is much smaller.

To accelerate finding the solutions of equations 20 and 21 we developed the following practical scheme. For an initial angle set we find the torques $\frac{\partial F(T)}{\partial \theta_i}$ from DFT-DLM and equation 13, and also calculate $\frac{\partial}{\partial \theta_j}\frac{\partial F(T)}{\partial \theta_i}$ by finite differences. We then use a Newton method to find the set of angles which would satisfy equations 20 or 21 if $\frac{\partial F(T)}{\partial \theta_i}$ were linear. This new angle set is then fed into a new set of DFT-DLM calculations, and the whole cycle iterated to convergence. We found this scheme to be efficient in limiting the number of computationally-expensive DFT-DLM calculations required. We stress that no linear approximation is made on the end solution, only during the Newton procedure to provide a guess for the next angle set.

## MEASUREMENT OF $K_1$ VERSUS TEMPERATURE FOR $GdCo_5$

Magnetization measurements were carried out on a platelet-shaped single crystal specimen of $GdCo_5$ in order to determine the temperature dependence of the anisotropy constant, $K_{\text{eff}}$. Details of the single crystal growth can be found in Ref. [7]. The single crystal was oriented and cut in such a way that the crystallographic $ab$ plane lies in the plane of the platelet with the $c$ axis normal to the plate.

Magnetization versus applied field curves were collected between 5 and 400 K using a Quantum Design Magnetic Property Measurement System (MPMS) magnetometer in applied fields $\mu_0 H$ up to 7 T. For measurements with the field applied along the easy axis, the single crystal was placed in a gel capsule containing Apiezon M grease, allowing the sample to rotate freely at room temperature in an applied field $\mu_0 H = 7$ T. Below room temperature, second quadrant demagnetization $M(H)$ data were then collected with the sample fixed in the frozen grease. Above room temperature the sample was free to rotate in the grease under field. These data were used to estimate the saturation magnetization ($M_0$) for fields applied along the easy axis. The values of $M_0$ agree well with previously published data, see for example, Ref. [18]. For measurements along the hard axis, the crystal was glued to a rigid sample holder. The crystal was then covered with a second rigid plate which was held in place using Kapton tape. These steps were taken to minimize any twisting of the sample in a magnetic field. Second quadrant demagnetization data were then collected at different temperatures to determine $M_{\text{ab}}$.

Figure 8 shows typical isothermal $M$ versus $H$ curves recorded at $T = 300$ K along the easy ($H \,//\, c$) and the hard ($H \perp c$) axes of magnetization. The magnetization along the easy axis (filled squares) saturates at higher fields and has a remanence of $0.38 \pm 0.01 \mu_\text{B}$/formula unit. The hard-axis magnetization (filled circles) is linear over the high field range. A non-zero remanent magnetization is attributed to a small (0 to 3°) misalignment of the crystal. Ideally, one would expect the hard-axis magnetization to pass through the origin. Following a procedure discussed in Ref. [19] we idealized the observed hard-axis magnetization by uniformly shifting the data (open circles).

To determine the anisotropy constant, $K_{\text{eff}}$, we plot the ratio $\eta = \frac{\frac{1}{2}BM_0}{M_{\text{ab}}/M_0}$ against the reduced magnetization $m = M_{\text{ab}}/M_0$ (see, for example, Fig. 9 plotted using the data shown in Fig. 8). The value of $\eta$ at $m = 0$ yields $K_{\text{eff}}$ [17]. At $T = 300$ K, $K_{\text{eff}}$ is found to be

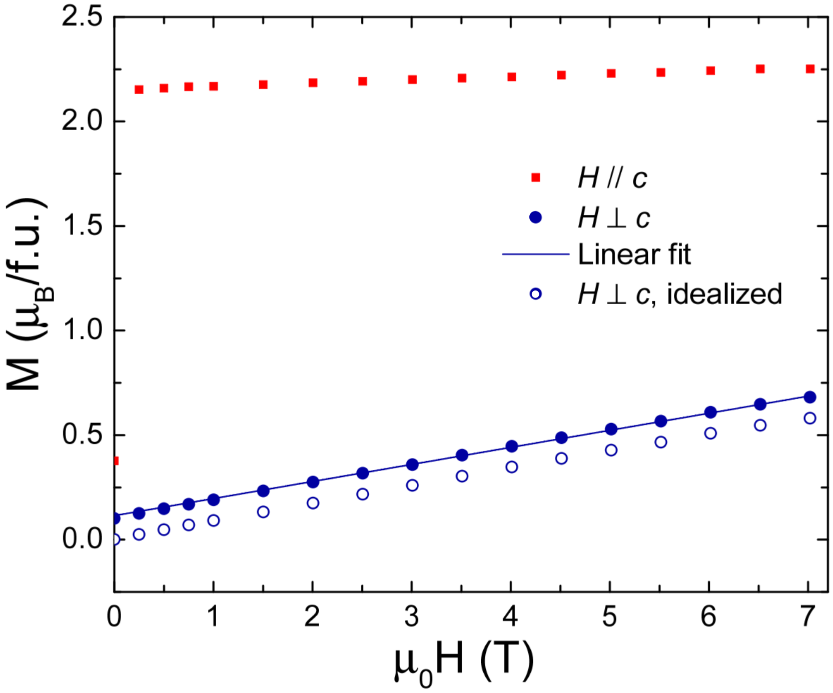


FIG. 8. $GdCo_5$ $M(H)$ curves for $H \,//\, c$ (filled squares) and $H \perp c$ (filled circles) at $T = 300$ K. The observed data for $H \perp c$ were idealized to pass through the origin (open circles).

$1.78 \pm 0.01$ meV/f.u. The variation of $K_{\rm eff}$ with temperature for $GdCo_5$ is presented in Fig. 3 of the main text. Measurements of $M(H)$ along the hard and easy axis were repeated several times producing values of $K_{\rm eff}(T)$ with a small spread indicated by the shaded region in Fig. 3 of the main text.

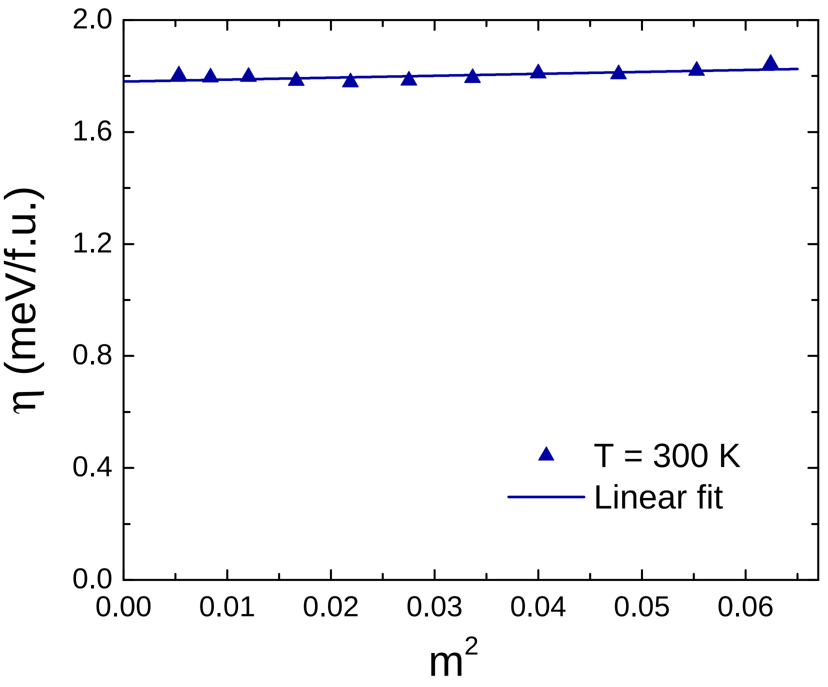


FIG. 9. $\eta$ versus $m^2$ at $T = 300$ K. A linear fit of the observed $GdCo_5$ data following the method described in Ref. [17] yields $K_{\mathrm{eff}} \sim 1.78 \pm 0.01$ meV/formula unit.


* c.patrick.1@warwick.ac.uk



[1] E. Bruno and B. Ginatempo, Phys. Rev. B **55**, 12946 (1997).

[2] B. L. Györffy, A. J. Pindor, J. Staunton, G. M. Stocks, and H. Winter, J. Phys. F: Met. Phys. **15**, 1337 (1985).

[3] P. Strange, J. Staunton, and B. L. Gyorffy, J. Phys. C: Solid State Phys. **17**, 3355 (1984).

[4] M. Däne, M. Lüders, A. Ernst, D. Ködderitzsch, W. M. Temmerman, Z. Szotek, and W. Hergert, J. Phys.: Condens. Matter **21**, 045604 (2009).

[5] S. H. Vosko, L. Wilk, and M. Nusair, Can. J. Phys. **58**, 1200 (1980).

[6] M. Lüders, A. Ernst, M. Däne, Z. Szotek, A. Svane, D. Ködderitzsch, W. Hergert, B. L. Györffy, and W. M. Temmerman, Phys. Rev. B **71**, 205109 (2005).

[7] C. E. Patrick, S. Kumar, G. Balakrishnan, R. S. Edwards, M. R. Lees, E. Mendive-Tapia, L. Petit, and J. B. Staunton, Phys. Rev. Materials **1**, 024411 (2017).

[8] O. Eriksson, B. Johansson, R. C. Albers, A. M. Boring, and M. S. S. Brooks, Phys. Rev. B

**42**, 2707 (1990).

[9] H. Eschrig, M. Sargolzaei, K. Koepernik, and M. Richter, Europhys. Lett. **72**, 611 (2005).

[10] L. Steinbeck, M. Richter, and H. Eschrig, Phys. Rev. B **63**, 184431 (2001).

[11] H. Ebert and M. Battocletti, Solid State Commun. **98**, 785 (1996).

[12] H. Ebert, "Fully relativistic band structure calculations for magnetic solids - formalism and application," in *Electronic Structure and Physical Properies of Solids: The Uses of the LMTO Method Lectures of a Workshop Held at Mont Saint Odile, France, October 2–5,1998*, edited by H. Dreyssé (Springer Berlin Heidelberg, Berlin, Heidelberg, 2000) pp. 191–246.

[13] P. Strange, *Relativistic Quantum Mechanics* (Cambridge University Press, 1998).

[14] W. Sucksmith and J. E. Thompson, Proc. Royal Soc. A **225**, 362 (1954).

[15] R. Radwaski, Physica B+C **142**, 57 (1986).

[16] R. Ballou, J. Deportes, and J. Lemaire, J. Magn. Magn. Mater. **70**, 306 (1987).

[17] J. Alameda, J. Deportes, D. Givord, R. Lemaire, and Q. Lu, J. Magn. Magn. Mater. **15**, 1257 (1980).

[18] M. D. Kuz'min, Y. Skourski, D. Eckert, M. Richter, K.-H. Müller, K. P. Skokov, and I. S. Tereshina, Phys. Rev. B **70**, 172412 (2004).

[19] K. Strnat, G. Hoffer, J. Olson, and W. Ostertag, J Appl. Phys. **38**, 3 (1967).
